# Supplementary material for: Molecular Excited State Calculations with Adaptive Wavefunctions on a Quantum Eigensolver Emulation: Reducing Circuit Depth and Separating Spin States
Source: arXiv:2105.10275 source file (2021-05-21)
Supplement: Supplementary file 1 [file appendix.tex]

\chapter{Appendix: Quantum Computing Overview} \label{section:quantumcompov}
    A digital \textit{quantum computer} is a programmable computer operating on quantum mechanical units of binary information (\textit{qubits}).
    It presents a unique computing architecture from conventional computing because qubits can exist in superposition, where the quantum state of a qubit $\ket{\psi}$ captures the probabilities $P_0$, $P_1$ associated with it being in the $\ket{0}$ state or the $\ket{1}$ state:
    \begin{equation}
        \ket{\psi} = c_0\ket{0} + c_1\ket{1}, \quad \text{where } P_0 = |c_0|^2 \quad  P_1 = |c_1|^2
    \end{equation}
    and can be made to entangle with each other, where the value of one qubit influences the value of another;
    consider generating the following example quantum state
    \footnote{
        Sometimes endearingly named the ``cat-state", after Einstein and Schr\"{o}dinger's infamous thought experiment.
    } 
    from 2 qubits:
    \begin{equation}
        \ket{\psi} = \frac{\ket{00}+\ket{11}}{\sqrt{2}}
    \end{equation}
    the qubits have equal probability of being both 0 or both 1 (the value of one qubit directly influences the value of the other).
    The power of these features can be appreciated when one considers a \textit{quantum register} with $N$ qubits;
    information about each computational basis vector i.e. each of the $2^N$ possible configurations of the qubits, is simultaneously captured by the quantum state of the $N$ qubits $\ket{\psi}$:
    \begin{equation}
        \ket{\psi} = c_0\ket{00\dots000} + c_1\ket{00\dots001} +  \dots + c_{2^N}\ket{11\dots111}
    \end{equation}
    $\ket{\psi}$ is a vector in the \textit{Fock space} i.e. the space spanned by the computational basis vectors $\{ \ket{x_1, x_2 \dots x_N} \}$ where $x_i \in \{0,1\}$. 

    Manipulation of the qubit quantum state $\ket{\psi}$, or \textit{quantum information}, can in effect process the information associated with every computational basis vector at once.
    The equivalent procedure in a classical machine will require memory of $2^N$ classical registers each with $N$ bits, as opposed to only $N$ qubits.
    A quantum program based on such architecture would typically have the following workflow:
    \begin{enumerate}
        \item Map the problem of interest into quantum information.
        \item Process the quantum information by manipulating the qubits, using a series of programmable unitary \textit{quantum logic gates} (see Appendix \ref{appendix:gates} for overview on quantum gates).
        An assembled sequence of quantum logic gates is a \textit{quantum circuit}.
        \item When the computation is deemed complete, information is extracted from the qubits through some form of measurement of the qubits, which in most types of calculations collapses the quantum state and destroys the quantum information.
    \end{enumerate}
    \begin{figure}[h!]
        \centering
        \begin{subfigure}[c]{0.3\textwidth}
            \centering
            \includegraphics[scale=0.22]{images/Bloch-Sphere.png}
        \end{subfigure}%
        \begin{subfigure}[c]{0.7\textwidth}
            \centering
            \includegraphics[scale=0.28]{images/qprogram.jpg}
        \end{subfigure}
        \caption[]{(LEFT) A Bloch sphere which shows how the state $\ket{\psi}$ of a single qubit can be $\ket{0}$, $\ket{1}$ or any superposition in between.
        (RIGHT) The general workflow of a quantum program running on a digital quantum computer.
        }
    \end{figure}

    Not all problems can be mapped onto quantum information and processed; in fact, not all computation will benefit from translation to a \textit{Quantum Processing Unit} (QPU).
    But where they can be applied, quantum computing has the potential to provide a polynomial speedup advantage.
    This ranges from rapid integer factorisation which is the basis of RSA encryptions\cite{Shor1995}, to provably optimal database search algorithms\cite{Grover1996}.
    
    Many of these algorithms require thousands of fault-tolerant logical qubits
    \footnote{
        At the time of writing, all proposed methods of qubit fault-correction requires a large overhead of dramatically more qubits:
        To maintain thousands of logical qubits, current theories project a requirement of millions of qubits more for error correction\cite{Endo2018}.
    }
    and circuits running on long \textit{coherence times} i.e. the duration within which a device can maintain the superposition of quantum information without premature collapse due to noise.
    This calls for near Fault-Tolerant Quantum (FTQ) computing capabilities, which will likely take years if not decades to realise on account of the delicate, noise-prone nature of quantum technologies.
    
    Nevertheless, in recent years, advances in solid state physics and quantum optics has initiated the ‘quantum-race’, where commercial and academic stakeholders alike are building the first functional QPUs\cite{Wright2019,Webb2018}.
    These nascent programmable machines have extremely modest computational power, with 53 noisy qubits being the current record for the largest quantum register\cite{Arute2019}, and very short coherence times that optimistically only allow for roughly $O(10^2-10^3)$ two-qubit gates on average\cite{Barends2014}.
    Despite these limitations, in some cases these devices are capable of computation faster than the equivalent action simulated on a classical computer, most clearly shown in the recent demonstration of quantum advantage for a proof-of-concept algorithm\cite{Arute2019}.
    Collectively, these machines are known as Noisy Intermediate-Scale Quantum (NISQ) computers\cite{McArdle2018}.

\chapter{Appendix: Quantum Gates Overview} \label{appendix:gates}
    Classical logic gates are electronic circuits which processes incoming bits of signal and returns a value.
    Quantum logic gates are controlled perturbations which change the state of qubits.
    Mathematically they are unitary transformations that act on the qubit space.
    The probability of a particular qubit state being measured depends therefore on how the qubits have been manipulated by these gates.

    In classical computing, any logic gate may be constructed from the NAND gate, and a computer being able to implement such a universal set is a universal computer.
    In a universal quantum computer, any logic gate may be constructed from the set of all the single qubit gates and any 2-qubit entangling gate.
    This work involves the simulation of a universal quantum computer.
    The following is an overview of the gates involved in electronic structure calculations

    The Hadamard gate $H$ is a single qubit gate that generates the simplest superposition in a qubit:
    \begin{figure}[h!]
        \centering
        \begin{subfigure}[c]{0.3\textwidth}
            \centering
            \vspace{1cm}
            \begin{quantikz}
            && \gate{H} & \qw \\
            \end{quantikz}
        \end{subfigure}%
        \begin{subfigure}[c]{0.3\textwidth}
            \centering
            \begin{align*}
                \ket{0} \rightarrow& \frac{1}{\sqrt{2}} (\ket{0} + \ket{1}) \\
                \ket{1} \rightarrow&  \frac{1}{\sqrt{2}} (\ket{0} - \ket{1})
            \end{align*}
        \end{subfigure}%
        \begin{subfigure}[c]{0.3\textwidth}
            \centering
            \begin{equation}
            H = \frac{1}{\sqrt{2}} \begin{bmatrix} 1 & 1 \\ 1 & -1 \end{bmatrix}
            \end{equation}
        \end{subfigure}
    \end{figure}
    
    Another important set of of single qubit gates are the Pauli matrices.
    The Pauli $X$ ($\sigma^x_i$) gate is the quantum equivalent of the NOT gate:
    \begin{figure}[h!]
        \centering
        \begin{subfigure}[c]{0.3\textwidth}
            \centering
            \vspace{1cm}
            \begin{quantikz}
            && \gate{X} & \qw \\
            \end{quantikz}
        \end{subfigure}%
        \begin{subfigure}[c]{0.3\textwidth}
            \centering
            \begin{align*}
                \ket{0} \rightarrow& \ket{1} \\
                \ket{1} \rightarrow& \ket{0}
            \end{align*}
        \end{subfigure}%
        \begin{subfigure}[c]{0.3\textwidth}
            \centering
            \begin{equation}
            X = \begin{bmatrix} 0 & 1 \\ 1 & 0 \end{bmatrix}
            \end{equation}
        \end{subfigure}
    \end{figure}

    The Pauli $Y$ ($\sigma^y_i$) gate rotates a qubit about the $y$-axis of the Bloch sphere by $\pi$ radians:
    \begin{figure}[h!]
        \centering
        \begin{subfigure}[c]{0.3\textwidth}
            \centering
            \vspace{1cm}
            \begin{quantikz}
            && \gate{Y} & \qw \\
            \end{quantikz}
        \end{subfigure}%
        \begin{subfigure}[c]{0.3\textwidth}
            \centering
            \begin{align*}
                \ket{0} \rightarrow&  i\ket{1} \\
                \ket{1} \rightarrow&  -i\ket{0}
            \end{align*}
        \end{subfigure}%
        \begin{subfigure}[c]{0.3\textwidth}
            \centering
            \begin{equation}
            Y = \begin{bmatrix} 0 & -i \\ i & 0 \end{bmatrix}
            \end{equation}
        \end{subfigure}
    \end{figure}
    
    The Pauli $Z$ ($\sigma^z_i$) gate flips the phase by rotating a qubit about the $z$-axis of the Bloch sphere by $\pi$ radians:
    \begin{figure}[h!]
        \centering
        \begin{subfigure}[c]{0.3\textwidth}
            \centering
            \vspace{1cm}
            \begin{quantikz}
            && \gate{Z} & \qw \\
            \end{quantikz}
        \end{subfigure}%
        \begin{subfigure}[c]{0.3\textwidth}
            \centering
            \begin{align*}
                \ket{0} \rightarrow& \ket{0} \\
                \ket{1} \rightarrow& -\ket{1}
            \end{align*}
        \end{subfigure}%
        \begin{subfigure}[c]{0.3\textwidth}
            \centering
            \begin{equation}
            Z = \begin{bmatrix} 1 & 0 \\ 0 & -1 \end{bmatrix}
            \end{equation}
        \end{subfigure}
    \end{figure}

    \newpage
    Single qubit rotation gates can be parameterised over all three dimensions of the Bloch sphere.
    One example is the single qubit rotation gate, which takes in a parameter of $\theta$:
    \begin{figure}[h!]
        \centering
        \begin{subfigure}[c]{0.3\textwidth}
            \centering
            \vspace{0.7cm}
            \begin{quantikz}
            && \gate{R(\theta)_O} & \qw \\
            \end{quantikz}
        \end{subfigure}%
        \begin{subfigure}[c]{0.4\textwidth}
            \centering
            \begin{equation}
                \begin{split}
                    R(\theta)_{X,Y,Z} &= e^{-\frac{i\theta}{2}}e^X e^Y e^Z\\
                    R(\theta)_{O} &= e^{-\frac{i\theta O}{2}} \\
                \end{split}
                \end{equation}
        \end{subfigure}
    \end{figure}

    Finally, the 2-qubit controlled-NOT (CNOT) gate is the only entangling gate used.
    It behaves like a classical CNOT gate: If the first qubit is in the $\ket{0}$ state the zeroth qubit is not flipped, whereas if the first qubit is $\ket{1}$ the second qubit is flipped.
    \begin{figure}[h!]
        \centering
        \begin{subfigure}[c]{0.3\textwidth}
            \centering
            \vspace{1cm}
            \begin{quantikz}
            && \ctrl{1} & \qw \\
            && \targ{} & \qw
            \end{quantikz}
        \end{subfigure}%
        \begin{subfigure}[c]{0.3\textwidth}
            \centering
            \begin{equation*}
                \begin{split}
                    |00\rangle&\rightarrow |00\rangle \\
                    |01\rangle&\rightarrow |01\rangle \\
                    |10\rangle&\rightarrow |11\rangle \\
                    |11\rangle&\rightarrow |10\rangle \\
                    \end{split}
            \end{equation*}
        \end{subfigure}%
        \begin{subfigure}[c]{0.4\textwidth}
            \centering
            \begin{equation}
            \text{CNOT} = \begin{bmatrix}1&0&0&0\\0&1&0&0\\0&0&0&1\\0&0&1&0\end{bmatrix}
            \end{equation}
        \end{subfigure}
    \end{figure}

    The novelty of quantum gates lie not in their ability to flip discrete $\ket{0}$ or $\ket{1}$ values, but rather in their ability to also manipulate a qubit that is in superposition $\ket{\psi}$.
    The resulting modified superposition will behave according to the corresponding matrix operation.

\chapter{Appendix: State Preparation Techniques}\label{appendix:stateprep}
VQE is not the only quantum state preparation; in fact it is a relatively new invention.
The following are two other methods of encoding molecular wavefunction and finding eigenenergies from a quantum computer.
Although they have been around for some time, they require long circuits and are not feasible in near-term technology.

\textbf{Quantum Phase Estimation} (QPE)
        is a powerful QPU primitive\cite{Dorner2009} found in many quantum programs.
        In the context of electronic structure, it returns near exact measurements of energy eigenvalues $E_\alpha$ (with probability $|c_\alpha|^2$) for a given Hamiltonian, from only a initial qubit state (e.g. $\ket{\psi_\text{HF}}$) of non-negligible overlap with the desired state. 
        However a FTQ computing level of resource is required to estimate energies accurately, and is not viable with near-term quantum technologies.
    
    \textbf{Time Evolution State Preparation Methods}
        adapt established classical chemistry concepts such as the adiabatic theorem\cite{Reiner2019} and imaginary time evolution\cite{McArdle2018a} to iteratively apply time-dependent operators on an initial state (e.g. $\ket{\psi_\text{HF}}$) until it evolves into a state matching the desired wavefunction, at which point the energy expectation is measured.
        Although these methods can potentially converge to any arbitrary electronic eigenstate without having determined lower energy states, solutions converge at large time steps thus require circuits longer than current coherence time can handle.
